# Supplementary material for: Hash Adaptive Bloom Filter
Source: arXiv:2106.07037 source file (2021-06-13)
Supplement: Supplementary file 1 [file appendix.tex]

\section{appendix}
\label{sec:appendix}

\subsection{Proof on Lemma 4.1 and Lemma 4.2}
\textbf{Lemma \ref{lemma:1}} $\forall u \in V, p \in H_0, 0\leq p(u) \leq 1$, have the following relation:
\begin{align}
\label{equa:appendixl1-1}
\prod \limits_{p\in H_0}(1-p(u)) \geq 1- \sum \limits_{p\in H_0}p(u).
\end{align}

\begin{proof}
Let $p_i$ be the distribution of the hash function $h_i$, then Equation (\ref{equa:appendixl1-1}) can be expressed as:
\begin{align}
\label{equa:appendixl1-2}
\prod \limits_{i = 0}^{k}(1-p_i(u)) \geq 1- \sum \limits_{i = 0}^{k}p_i(u).
\end{align}

We denote Equation (\ref{equa:appendixl1-2}) as $\Psi$.
Next we use mathematical induction to prove $\Psi$, obviously it holds when $k=0$, we assume that $\Psi$ holds when $k=\alpha-1$, then we have $\prod \limits_{i = 0}^{\alpha-1}(1-p_i(u)) \geq 1- \sum \limits_{i = 0}^{\alpha-1}p_i(u)$ and we can get:

\begin{align}
\label{equa:appendixl1-3}
\prod \limits_{i = 0}^{\alpha}(1-p_i(u)) & = (1-p_\alpha(u))\prod \limits_{i = 0}^{\alpha-1}(1-p_i(u))\notag\\
&=\prod \limits_{i = 0}^{\alpha-1}(1-p_i(u)) - p_\alpha(u) \prod \limits_{i = 0}^{\alpha-1}(1-p_i(u))\notag\\
& \geq 1- \sum \limits_{i = 0}^{\alpha-1}p_i(u) - p_\alpha(u) \prod \limits_{i = 0}^{\alpha-1}(1-p_i(u))\notag\\
& \geq 1- \sum \limits_{i = 0}^{\alpha}p_i(u).
\end{align}
Therefore, $\Psi$ holds when $k=\alpha$, this completes the proof.
\end{proof}

\textbf{Lemma \ref{lemma:2}} $\forall 0\leq x\leq 1$, Function $f(x) = \frac{|S|\cdot x}{\frac{1}{(1-x)^{|S|}}-1}$
is a convex function.
\begin{proof}
We rewrite the $f(x)$ as follows:
\begin{align}
\label{equa:appendixl2-1}
 f(x) = & \frac{|S|\cdot x(1-x)^{|S|}}{1-(1-x)^{|S|}} = \frac{|S|\cdot (1-x)^{|S|}}{\sum \limits_{i = 0}^{|S|-1} (1-x)^i}
\end{align}

Let $\mu = 1-x$ and $\theta = |S|$, so $f(\mu) = \frac{\theta \mu^{\theta}}{\sum \limits_{i = 0}^{\theta-1} \mu^i}$, and we can derive $f'(\mu)$ as follows:

\begin{align}
\label{equa:appendixl2-2}
 f'(\mu) = & \theta\frac{\sum \limits_{i = \theta-1}^{2\theta-2}(2\theta-1-i)\mu^i}{(\sum \limits_{i = 0}^{\theta-1} \mu^i)^2} > 0
\end{align}

Since $f'(x) = \frac{\delta f(\mu)}{\delta \mu} \frac{\delta \mu}{\delta x} = -f'(\mu) < 0$, then we can derive $f''(\mu)$ as follows:
\begin{align}
\label{equa:appendixl2-3}
 f''(\mu)&  = \frac{\theta}{(\sum \limits_{i = 0}^{\theta-1} \mu^i)^4}((\sum \limits_{i = 0}^{\theta-1} \mu^i)^2 \sum \limits_{i = \theta-1}^{2\theta-2}i(2\theta-1-i)\mu^{i-1} \notag\\
  &-2\sum \limits_{i = 0}^{\theta-1} \mu^i\sum \limits_{i = 1}^{\theta-1}i \mu^{i-1}\sum \limits_{i = \theta-1}^{2\theta-2}(2\theta-1-i)\mu^i)\notag\\
  & = \frac{\theta}{(\sum \limits_{i = 0}^{\theta-1} \mu^i)^3}(\sum \limits_{i = 0}^{\theta-1} \mu^i \sum \limits_{i = \theta-1}^{2\theta-2}i(2\theta-1-i)\mu^{i-1} \notag\\
  &-2\sum \limits_{i = 0}^{\theta-1}i \mu^i\sum \limits_{i = \theta-1}^{2\theta-2}(2\theta-1-i)\mu^{i-1})
\end{align}

Next, we compare $\sum \limits_{i = 0}^{\theta-1}i \mu^i$ with $\frac{\theta-1}{2} \sum \limits_{i = 0}^{\theta-1}\mu^i$,

\begin{align}
\label{equa:appendixl2-4}
 & \frac{\theta-1}{2} \sum \limits_{i = 0}^{\theta-1}\mu^i - \sum \limits_{i = 0}^{\theta-1}i \mu^i \notag\\
 =& \sum \limits_{i = 0}^{\theta-1}(\frac{\theta-1}{2} - i)\mu^i \notag\\
 =& \sum \limits_{i = 0}^{\frac{\theta-1}{2}}(\frac{\theta-1}{2} - i)(\mu^i - \mu^{\theta - 1 - i})
\end{align}

Since $0\leq \mu \leq 1$, we have $\sum \limits_{i = 0}^{\theta-1}i \mu^{i}  < \frac{\theta-1}{2} \sum \limits_{i = 0}^{\theta-1}\mu^{i}$. According to Equation (\ref{equa:appendixl2-3}), we have:

\begin{align}
\label{equa:appendixl2-5}
f''(\mu) & > \frac{\theta}{(\sum \limits_{i = 0}^{\theta-1} \mu^i)^3}(\sum \limits_{i = 0}^{\theta-1} \mu^i \sum \limits_{i = \theta-1}^{2\theta-2}i(2\theta-1-i)\mu^{i-1} \notag\\
  &-(\theta-1) \sum \limits_{i = 0}^{\theta-1}\mu^{i}\sum \limits_{i = \theta-1}^{2\theta-2}(2\theta-1-i)\mu^{i-1})\notag\\
& = \frac{\theta}{(\sum \limits_{i = 0}^{\theta-1} \mu^i)^2}\sum \limits_{i = \theta-1}^{2\theta-2}(i-(\theta-1))(2\theta-1-i)\mu^{i-1}
\end{align}

Therefore, $f''(\mu) > 0$ and $f''(x) = \frac{\delta^2 f(\mu)}{\delta^2 \mu}(\frac{\delta \mu}{\delta x})^2 + \frac{\delta f(\mu)}{\delta \mu}(\frac{\delta^2 \mu}{\delta^2 x})= f''(\mu) > 0$. Since $f'(x)<0,f''(x)>0$, $f(x)$ is a convex function.

\end{proof}

\subsection{Analysis of $P'_c$}
%Next, we analyze $P'_c$.
%
To simplify the analysis, we assume that each bit in Bloom filter is set to $0$ with probability $p_0$ and $1$ with probability $ 1 - p_0$.
Note that we do not consider the case of $cost$ $exchange$.
When all buckets mapped by $e_{sk}$ through all hash functions in $H_c$ are \emph{conflict after adjustment}, we cannot adjust the hash functions of $e_{sk}$, so we get
\begin{align}
P'_c = 1 - \prod \limits_{h \in H_c(e_{sk})}(1-(1-p_0^{k-1})^{\chi(h(e_{sk}))}),
\end{align}
where $\chi(i)$ represents the number of keys in the $i^{th}$ bucket of $\Gamma$.
Moreover, according to average value inequality, we have
\begin{align}
1-P'_c \leq & (\frac{|H|-k - \sum \limits_{h \in H_c}(1-p_0^{k-1})^{\chi(h(e_{sk}))}}{|H|-k})^{|H|-k} \notag\\
 \leq & (1-\frac{1}{|H|-k}\sum \limits_{h \in H_c}(1-p_0^{k-1})^{\chi(h(e_{sk}))})^{|H|-k} \notag\\
\leq & (1-\prod \limits_{h \in H_c}(1-p_0^{k-1})^{\frac{\chi(h(e_{sk}))}{|H|-k}})^{|H|-k}.
\end{align}
It is easy to prove that: $ \forall 0<\alpha<1, \beta \in \mathbb{N}, (1-\alpha)^\beta < 1-\alpha ^\beta$, which is similar to Lemma \ref{lemma:1}, then we have
\begin{align}
1-P'_c < &  1-(1-p_0^{k-1})^{\sum \limits_{h \in H_c}\chi(h(e_{sk}))} \notag\\
P'_c > & (1-p_0^{k-1})^{\sum \limits_{h \in H_c}\chi(h(e_{sk}))}.
\end{align}
Since function $g''(x) = (1-p_0^{k-1})^{x}$ is a convex function, by the Jensen inequality, we get
\begin{align}
E(P'_c) > (1-p_0^{k-1})^{E(\sum \limits_{h \in H_c}\chi(h(e_{sk})))}.
\end{align}

Let $\psi = \sum \limits_{h \in H_c}\chi(h(e_{sk}))$, and we assume that $\forall h \in H, e_{sk} \in S$, for a certain unit $u$ in $V$, the probability that $u$ is mapped by $e_{sk}$ through $h$ is only determined by $p(u)$, so we have
\begin{align}
E(\psi) =& E(\sum \limits_{u = 1}^{m} \sum \limits_{p \in H_c}\chi(u)p(u)) = E(\sum \limits_{u = 1}^{m}\chi(u) \sum \limits_{p \in H_c}p(u)),
\end{align}
where $\chi(u) = |O|\sum \limits_{p' \in H_0}p'(u)$, for $\forall p_\alpha \in H_0$, $p_\gamma \in H_c$, $p_\alpha$ and $p_\gamma$ are independent of each other, we have
\begin{align}
E(\psi) =& \sum \limits_{u = 1}^{m}|O| E(\sum \limits_{p \in H_0}p(u)) \cdot E(\sum \limits_{p \in H_c}p(u)) \notag\\
<& \sum \limits_{u = 1}^{m} \frac{|O|}{4}(\sum \limits_{p \in H}E(p(u)))^2 = \frac{|O|\cdot |H|^2}{4m}.
\end{align}
Since $0 < (1-p_0^{k-1}) < 1$, then
\begin{align}
E(P'_c) > (1-p_0^{k-1})^{\frac{|O|\cdot |H|^2}{4m}}.
\end{align}
\red{
\subsection{Analysis of HABF Under Insertion Workloads}
In this subsection, we theoretically analyze the performance of HABF under insertion workloads.
Let the cost of the $i^{th}$ bit of Bloom filter be $\Theta'(i)$. %due to the limit of space size, we can only customize a small part of hash functions for massive inserted keys, we only consider the scenario that $\Theta'$ is skew.
If $\alpha$ keys have been inserted, the probability that a certain bit remains '0' is $(1-\frac{1}{m})^{k\alpha}$.}

\red{Thus, for Bloom filter, the overall cost of false positives in $O$ can be derived as
\begin{align}
C_{bf} = \sum \limits_{i = 1}^m (1-(1-\frac{1}{m})^{k\alpha})\Theta'(i).
\end{align}}

\red{For HABF, in this scenario, when a bit $x$ is set to `1', we compare its cost with the preset threshold $\tau$.
If $\Theta'(x) \geq \tau$, we try to customize the hash functions of inserted positive keys to avoid $x$ set to `1'.
We denote the probability that a bit $i$ is avoided $x$ set to `1' as $P(i)$, then for HABF, the overall cost of false positives in $O$ can be derived as
\begin{align}
\label{equa:dynamic3}
C_{habf} = \sum \limits_{i = 1}^m (1-(1-\frac{1}{m}+\frac{P(i)}{m})^{k\alpha})\Theta'(i).
\end{align}}

\red{As per Equation (\ref{equa:dynamic3}), it is obvious that $C_{habf} \leq C_{bf}$.
Since $(1-\frac{1-P(i)}{m}) < 1, \lim\limits_{\alpha\to+\infty}C_{habf} = \sum\limits_{i = 1}^m \Theta'(i)$, which means $C_{habf}$ will also tend to reach the max overall cost but at a lower speed.
Next we analyze $P$ in detail. We denote $P_c$ as the probability that a inserted key can be customized its hash functions successfully and $P_c$ as the probability that the customization results can be inserted into HashExpressor. For simplification, we assume that $P_c$ and $P_s$ are independent of each other, then we have
\begin{align}
\label{equa:dynamic4}
P(i) = Pr(\Theta'(i) > \tau)\cdot P_c\cdot P_s.
\end{align}
We set $\tau$ to the $h^{th}$ highest value in $\Theta'(i)$ for $i=1, 2, ..., m$, then $Pr(\Theta'(i) > \tau) = \frac{h}{m}$.
Considering $P_c$, for a inserted key $e$, and there are $|H_c|$ hash functions for selection, if there exists a hash function which can be used to mapped to a bit with cost below $\tau$, the customization is successful, then
%%
%In practical, only a small part of hash functions for massive inserted keys are customized, we assume the underly distribution of '1' is ideal uniform, then
\begin{align}
\label{equa:dynamic5}
P_c = 1-(\frac{h}{m})^{|H_c|}.
\end{align}
Considering $P_s$ related to the number of customized keys, which we denote as $t$, and according to Equation (\ref{equa:8}) and Lemma \ref{lemma:1}, we have
\begin{align}
\label{equa:dynamic6}
P_s  > (1-\frac{kt+k}{\omega})^k > 1-\frac{k^2(t+1)}{\omega}.
\end{align}
As per Equation (\ref{equa:dynamic4}), we have $E(t) = k\alpha\cdot \frac{h}{m}\cdot P_c \cdot E(P_s)$, then we can derive
\begin{align}
\label{equa:dynamic7}
E(P_s) > & 1-\frac{k^2(E(t)+1)}{\omega}\notag\\
>& 1-\frac{k^2( \frac{k\alpha hP_c}{m} \cdot E(P_s)+1)}{\omega}\notag\\
>& \frac{(\omega+k^2)m}{\omega m+k^3\alpha hP_c}.
\end{align}
As per Equation (\ref{equa:dynamic4}) and (\ref{equa:dynamic7}), then we have
\begin{align}
\label{equa:dynamic8}
E(P(i)) > \frac{(\omega+k^2)}{\frac{\omega m}{P_c h}+k^3\alpha}.
\end{align}}
